# Supplementary material for: StyleInject: Parameter Efficient Tuning of Text-to-Image Diffusion Models
Source: arXiv:2401.13942 source file (2024-05-10)
Supplement: Supplementary file 1 [file visu_supp_v2.pdf]

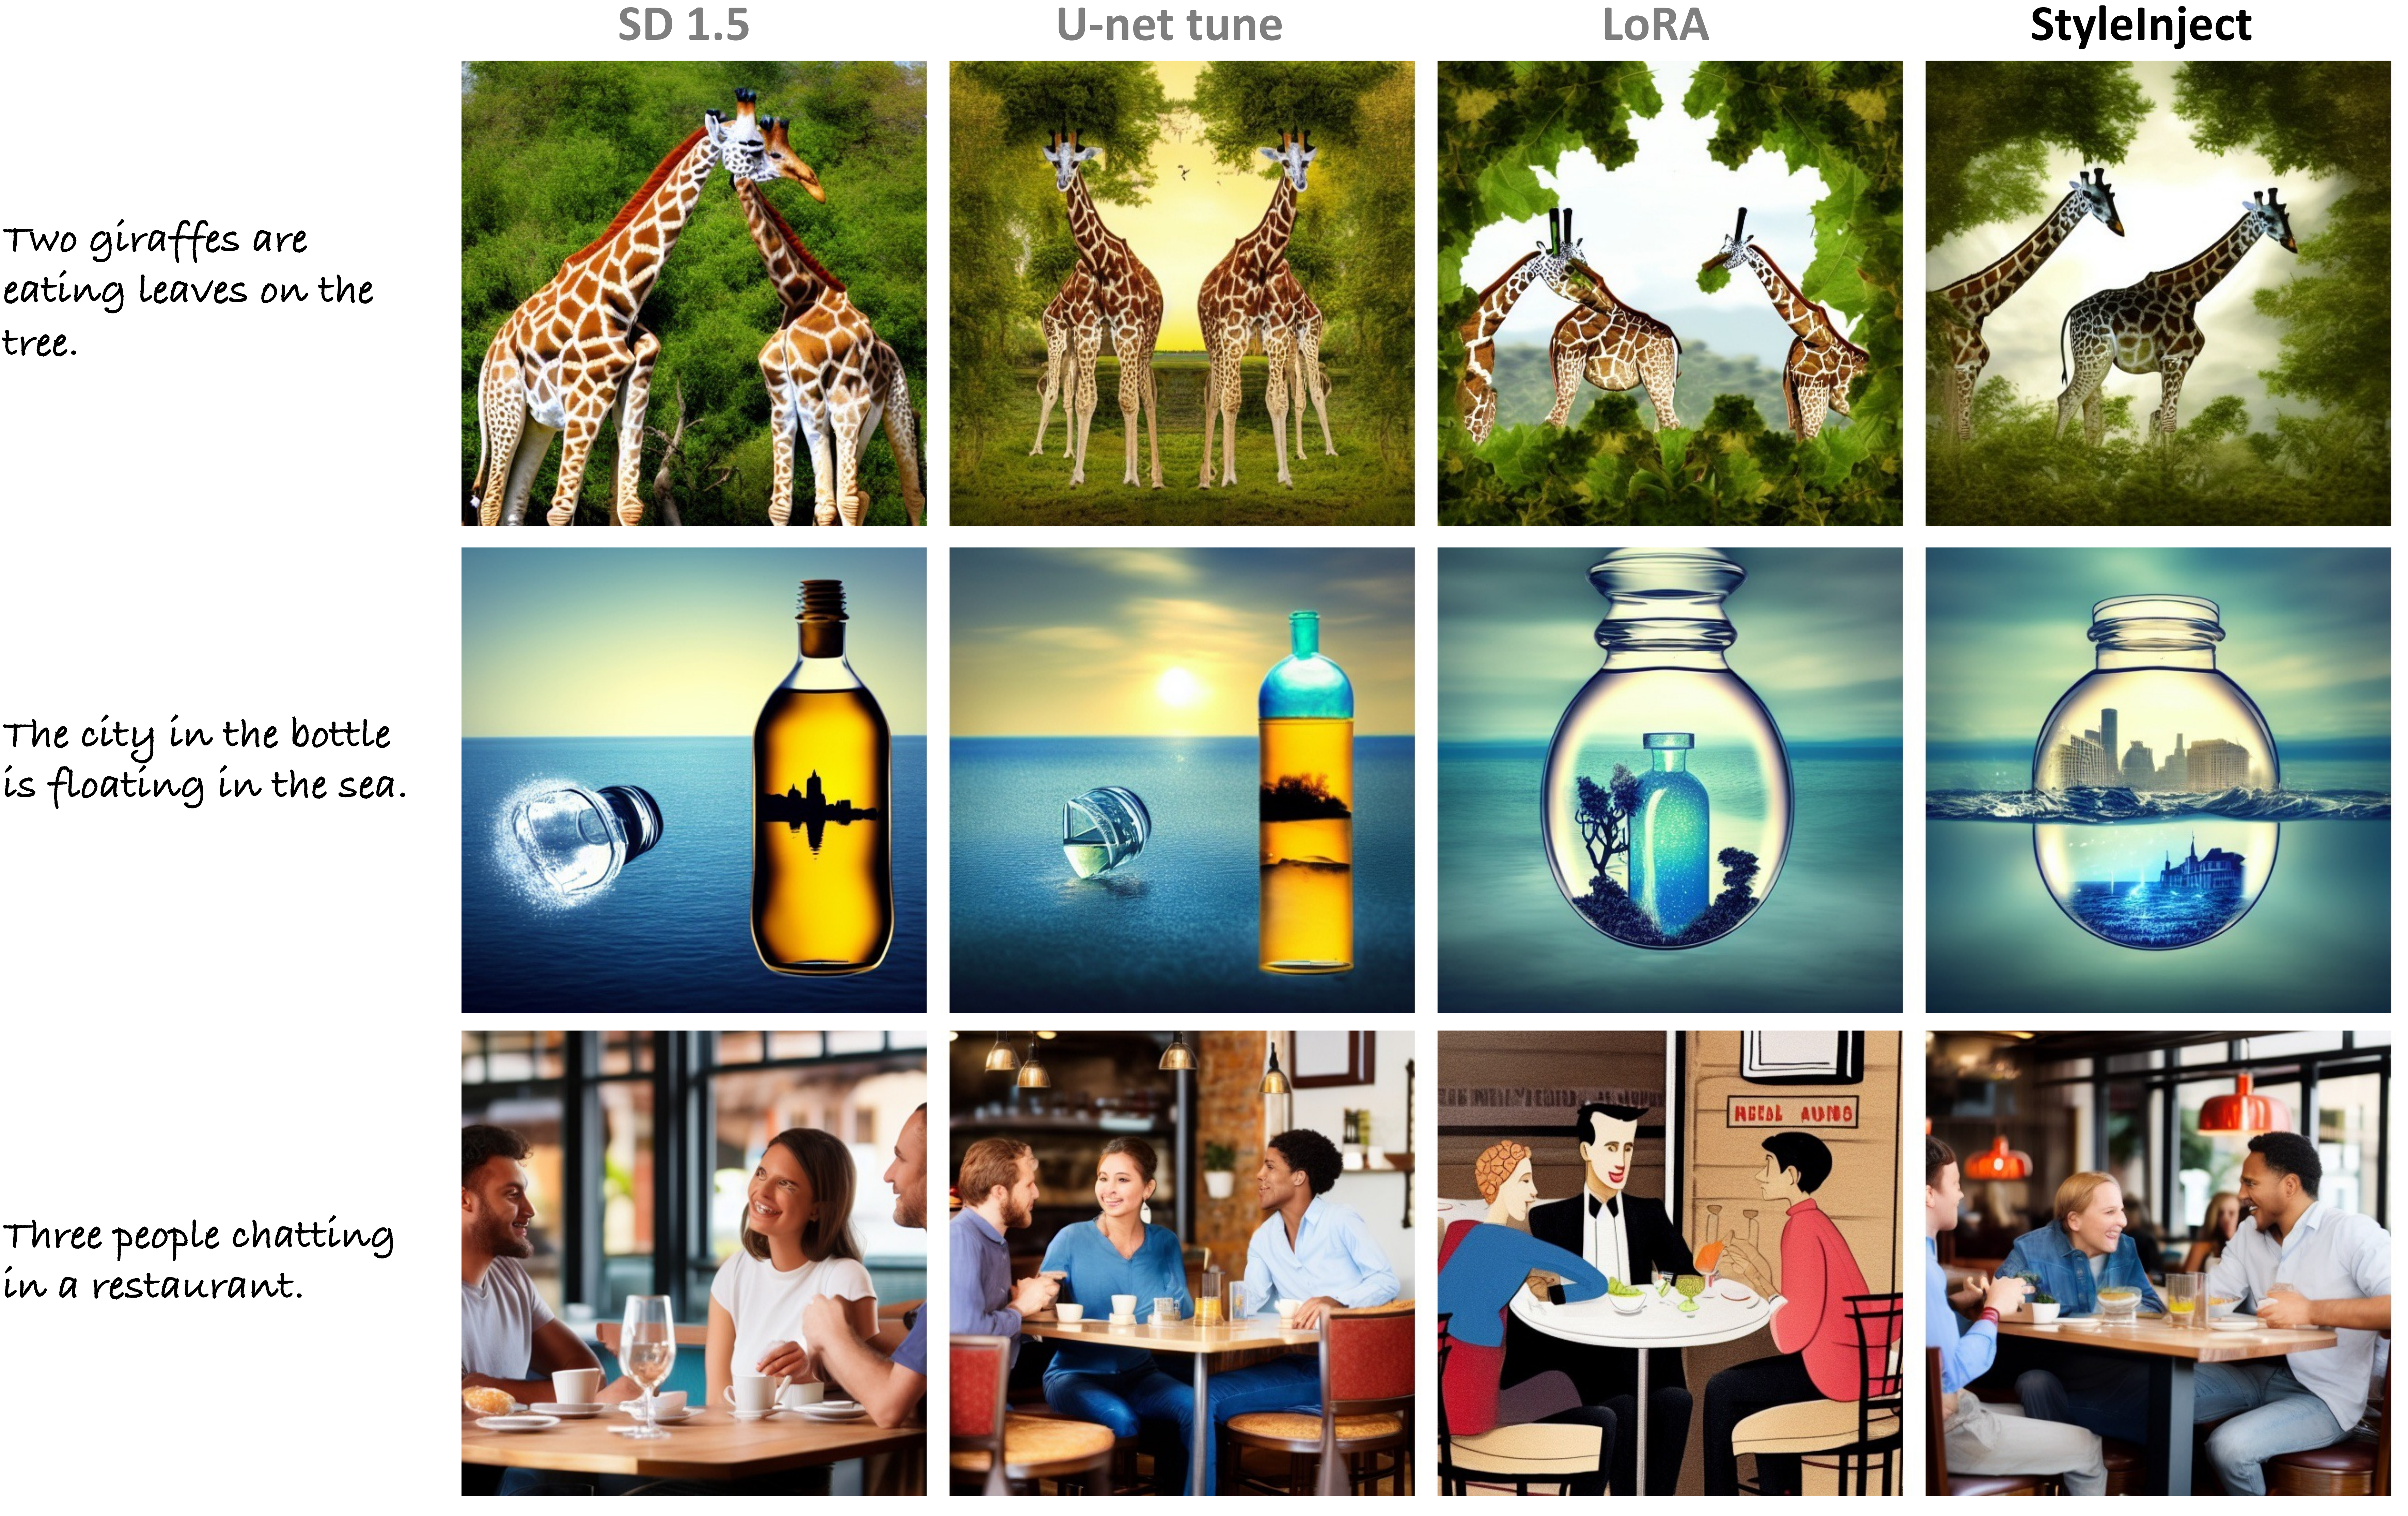
SD 1.5
U-net tune
LoRA
StyleInject
Two giraffes are eating leaves on the tree.
The city in the bottle is floating in the sea.
Three people chatting in a restaurant.

DreamShaper | SD 1.5 | U-net tune | LoRA | **StyleInject**

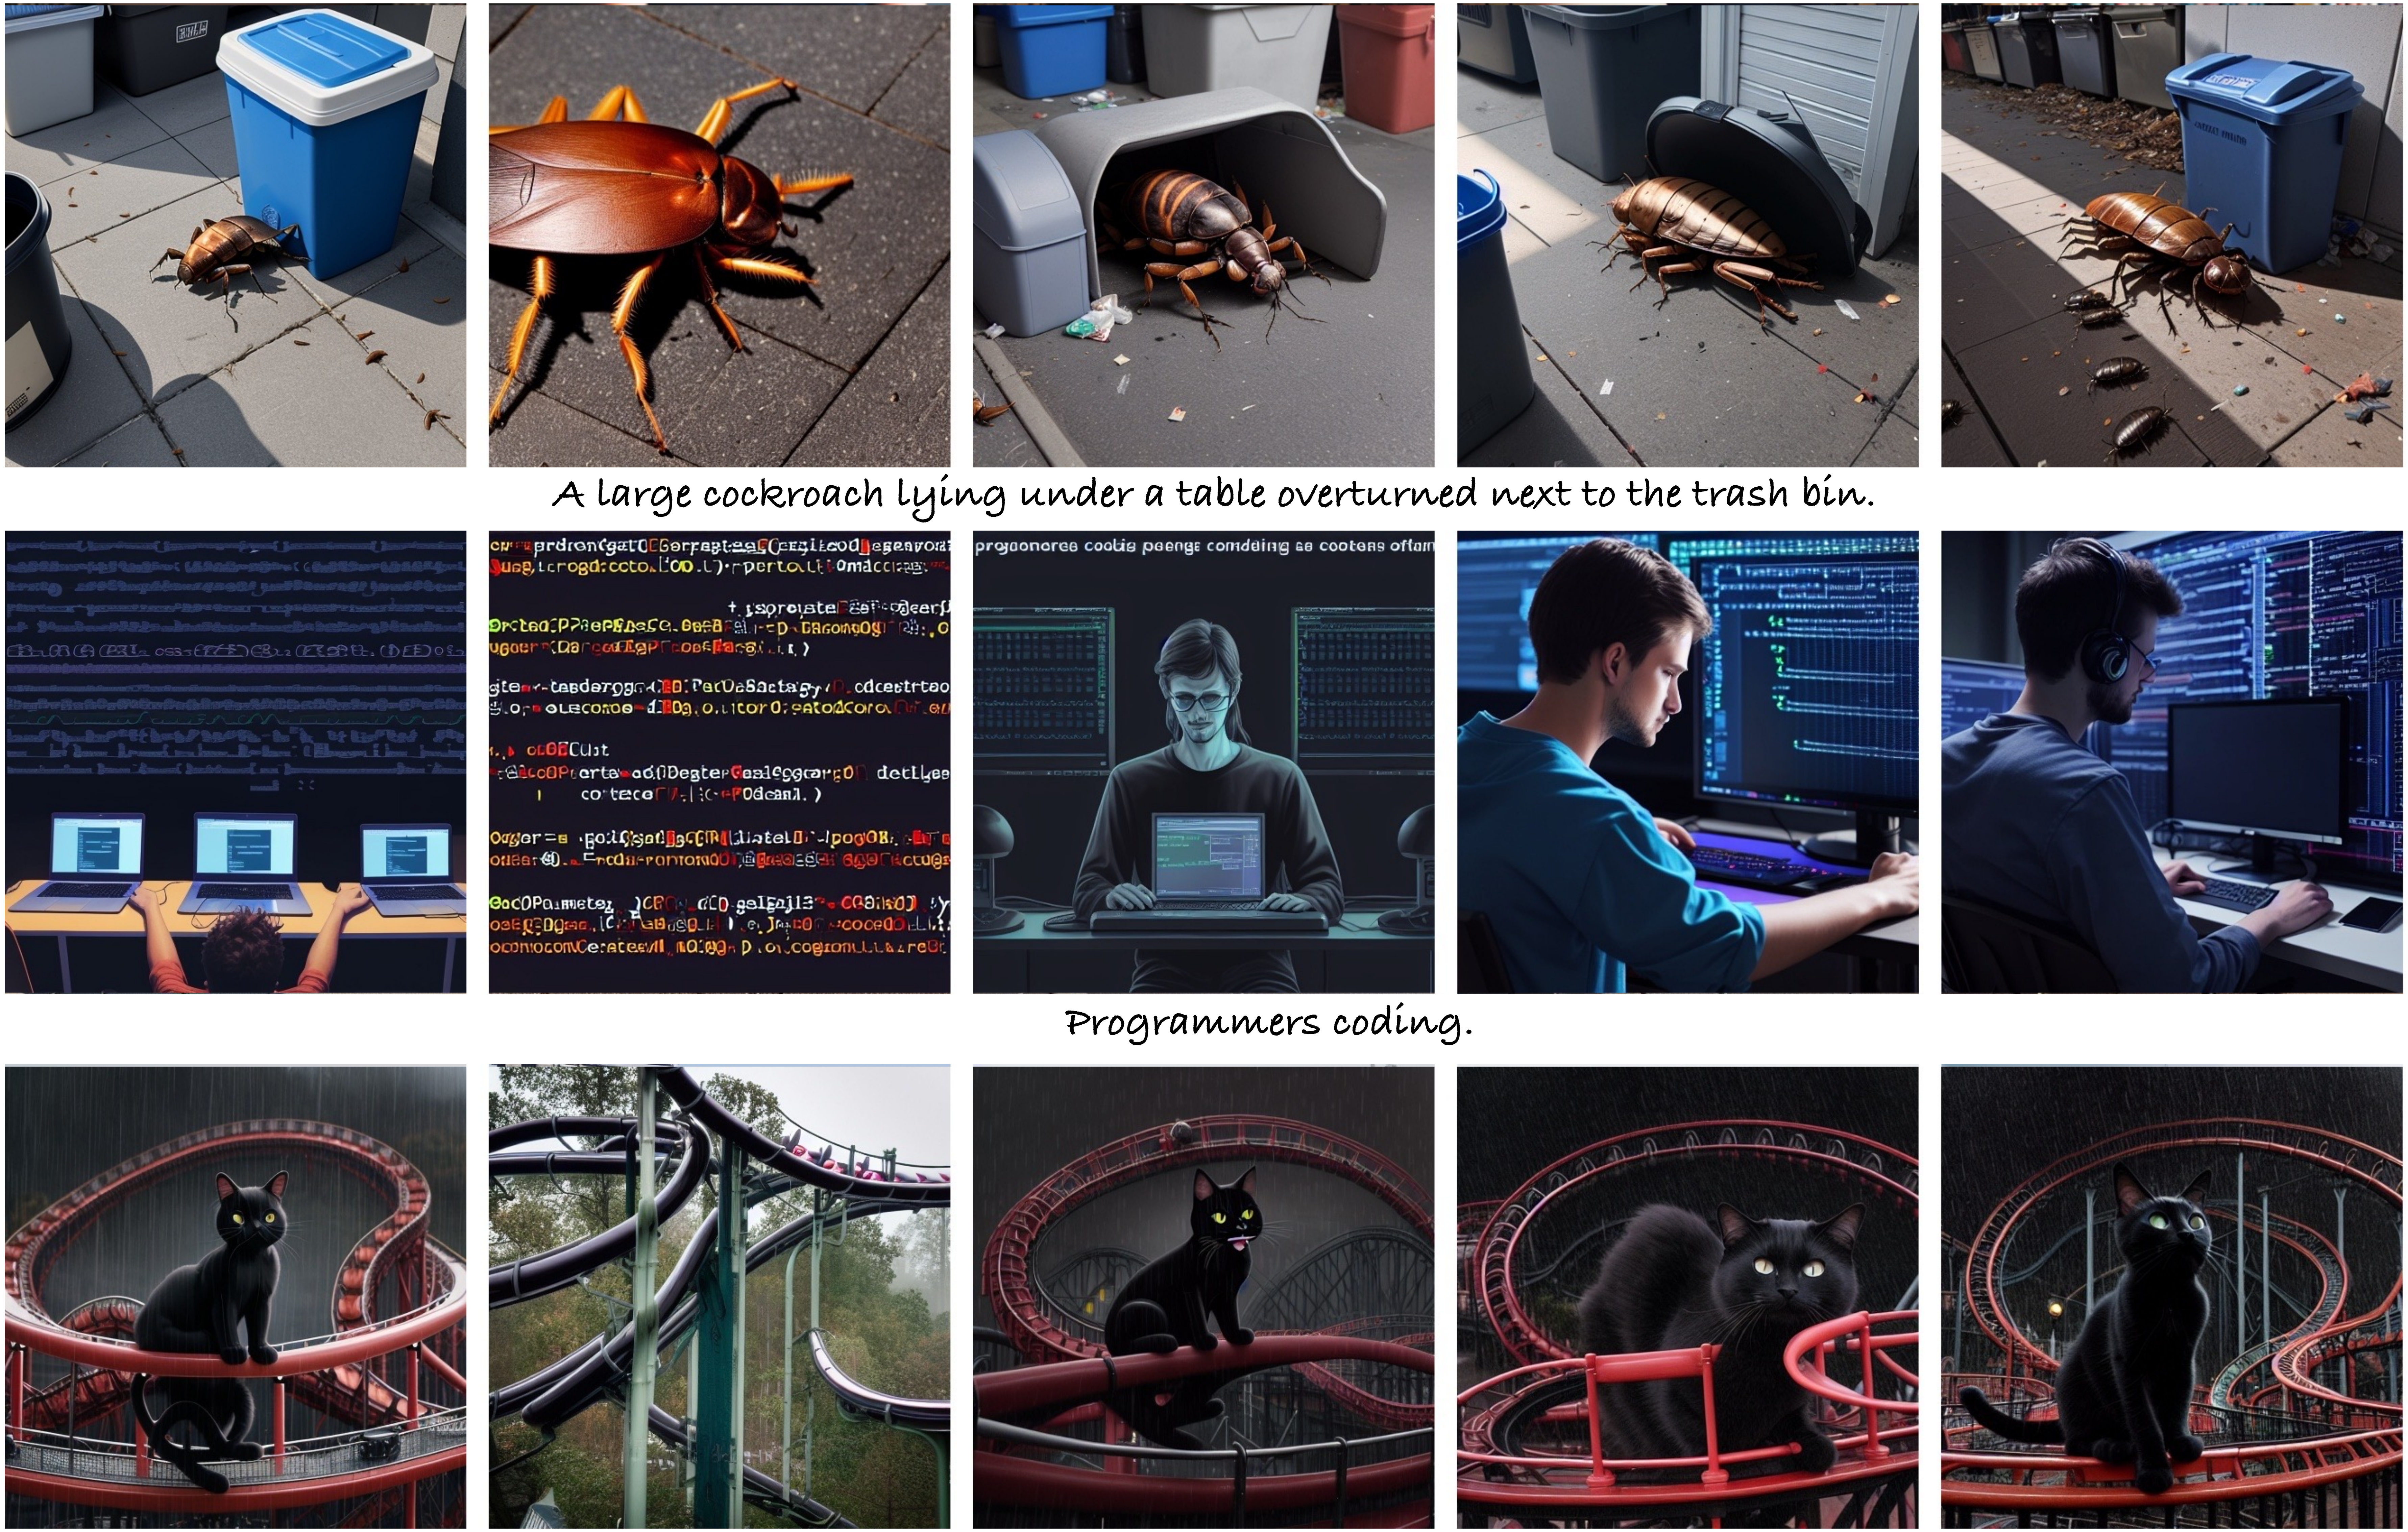

A large cockroach lying under a table overturned next to the trash bin.

Programmers coding.

A black cat sitting on the roller coaster rails.

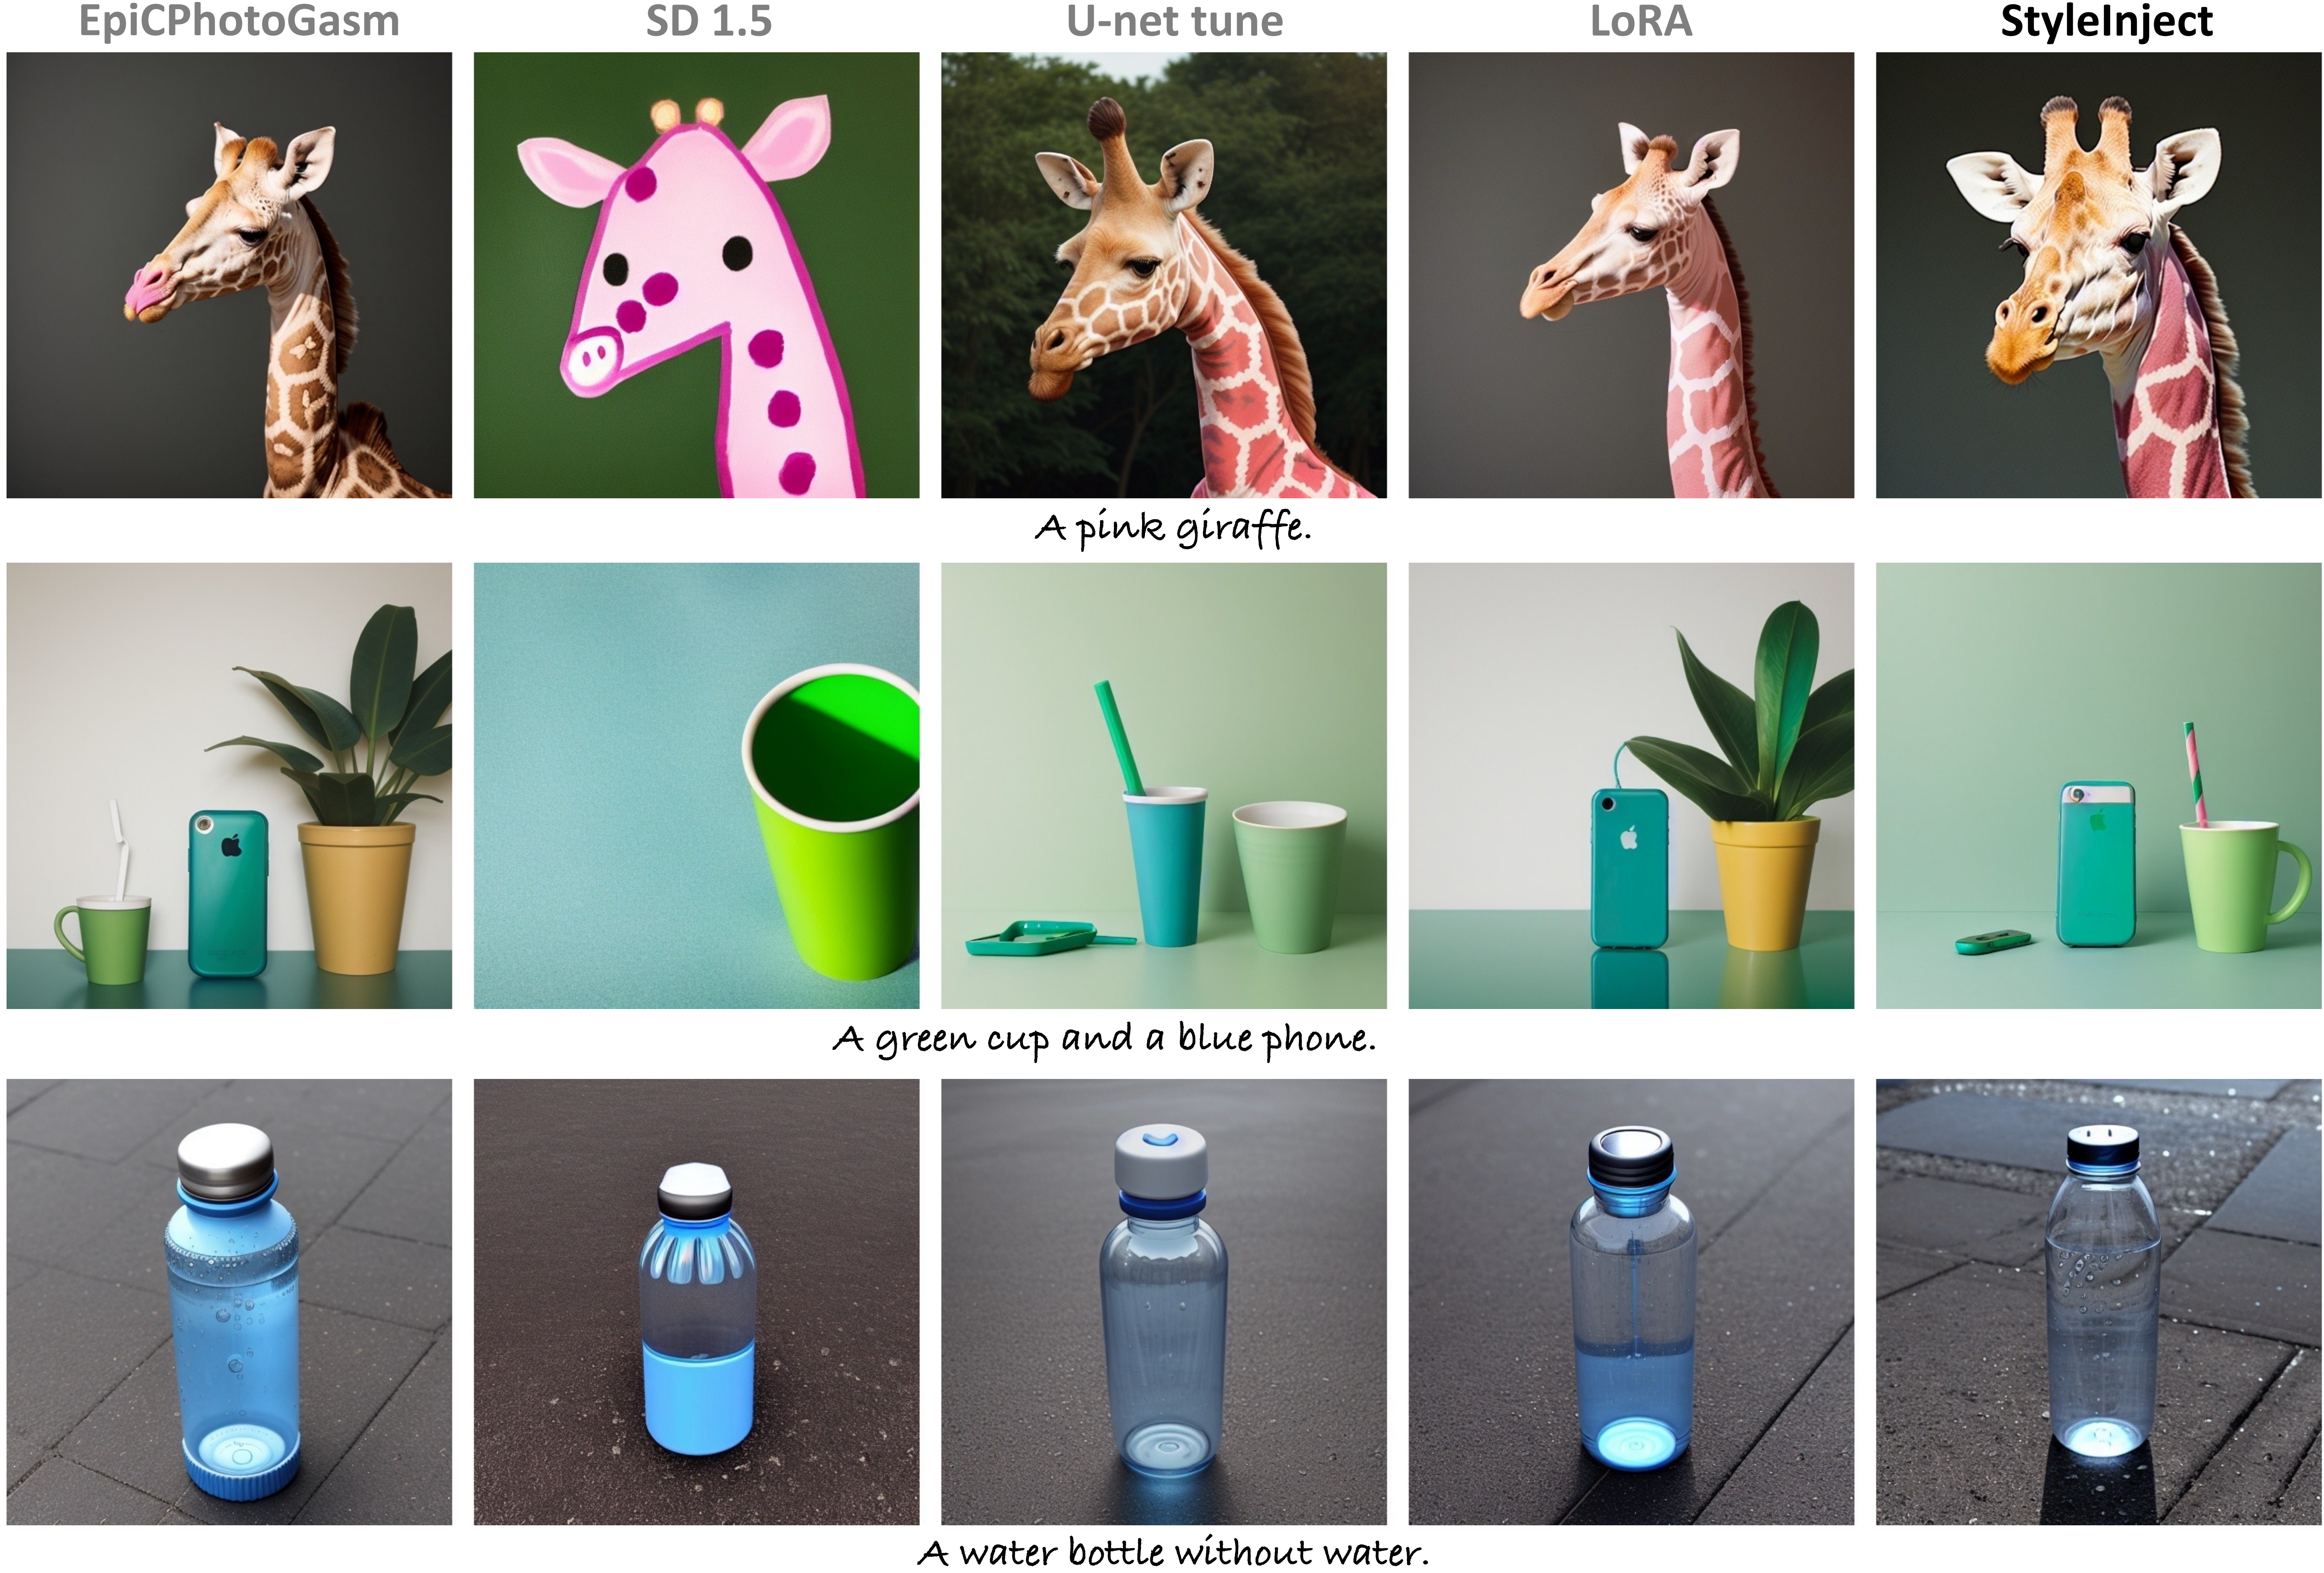
EpiCPhotoGasm
SD 1.5
U-net tune
LoRA
StyleInject
A pink giraffe.
A green cup and a blue phone.
A water bottle without water.

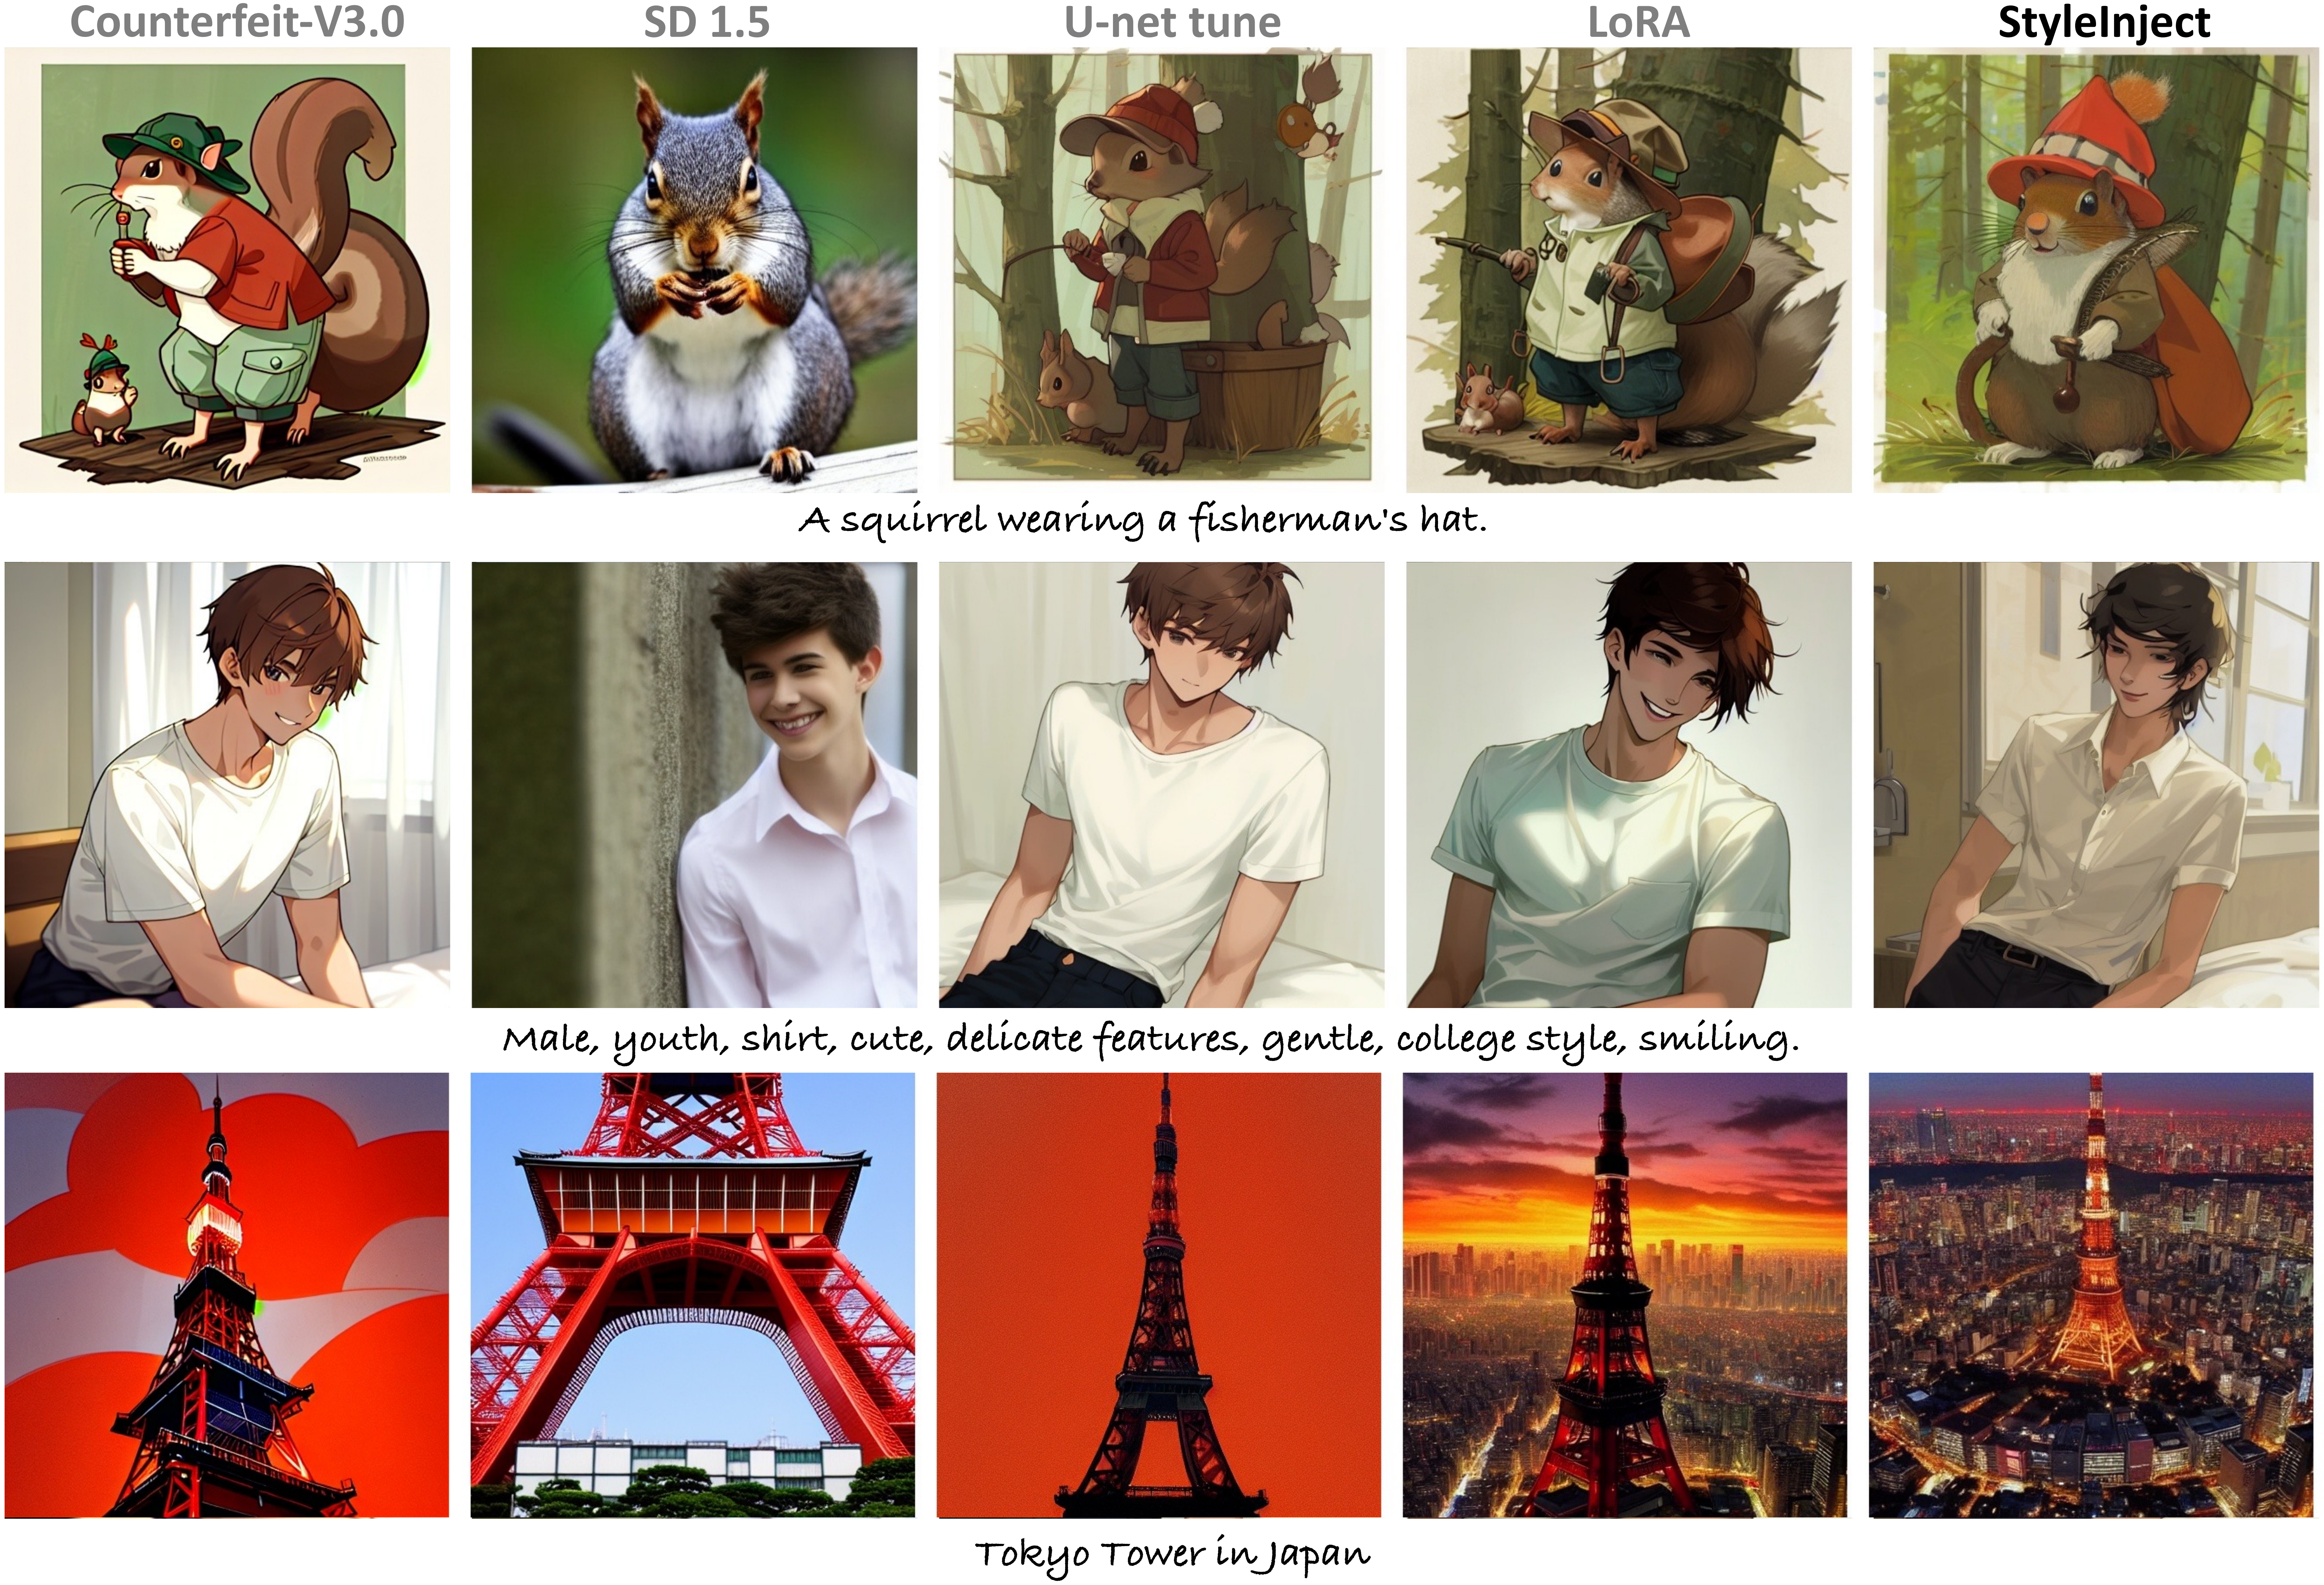
Counterfeit-V3.0
SD 1.5
U-net tune
LoRA
StyleInject
A squirrel wearing a fisherman's hat.
Male, youth, shirt, cute, delicate features, gentle, college style, smiling.
Tokyo Tower in Japan
